# Supplementary material for: On the Utility of Domain Modeling Assistance with Large Language Models
Source: arXiv:2410.12577 source file (2024-10-16)
Supplement: Supplementary file 1 [file ExperimentquestionnaireGoogleForms.pdf]

# Experiment questionnaire

Evaluation of the experiment

* Indicates required question

1. UserID *

2. Mode *

*Mark only one oval.*

- Automatic Suggestions *Skip to question 9*
- On request Suggestions *Skip to question 3*
- Completion at the end *Skip to question 6*

## On Request Mode

On a scale of 1 to 5, where 1 is the lowest value and 5 the highest value, please, respond to the following questions.

3. During the experiment, I felt... *

*Mark only one oval per row.*

| | 1 | 2 | 3 | 4 | 5 |
|---|---|---|---|---|---|
| **Confident** | ⬭ | ⬭ | ⬭ | ⬭ | ⬭ |
| **Creative** | ⬭ | ⬭ | ⬭ | ⬭ | ⬭ |
| **Confused** | ⬭ | ⬭ | ⬭ | ⬭ | ⬭ |
| **Guided towards a good solution** | ⬭ | ⬭ | ⬭ | ⬭ | ⬭ |
| **Productive** | ⬭ | ⬭ | ⬭ | ⬭ | ⬭ |
| **Slowed down** | ⬭ | ⬭ | ⬭ | ⬭ | ⬭ |

4. I found the tool... *

*Mark only one oval per row.*

| | 1 | 2 | 3 | 4 | 5 |
|---|---|---|---|---|---|
| **Easy-to-use** | ⬭ | ⬭ | ⬭ | ⬭ | ⬭ |
| **Good fit for the purpose** | ⬭ | ⬭ | ⬭ | ⬭ | ⬭ |
| **Intuitive** | ⬭ | ⬭ | ⬭ | ⬭ | ⬭ |
| **Slow** | ⬭ | ⬭ | ⬭ | ⬭ | ⬭ |
| **Visually appealing** | ⬭ | ⬭ | ⬭ | ⬭ | ⬭ |

5. I found the recommendations.... *

*Mark only one oval per row.*

| | 1 | 2 | 3 | 4 | 5 |
|---|---|---|---|---|---|
| **Complete** | | | | | |
| **Confusing** | | | | | |
| **Correct** | | | | | |
| **Credible** | | | | | |
| **Inconsistent** | | | | | |
| **Intuitive** | | | | | |
| **Stimulating (they gave me ideas I did not have)** | | | | | |
| **Useful** | | | | | |
| **Well-timed (they appeared right when I expected them)** | | | | | |

*Skip to question 12*

## Completion at end

On a scale of 1 to 5, where 1 is the lowest value and 5 the highest value, please, respond to the following question.

6. During the experiment, I felt... *

*Mark only one oval per row.*

| | 1 | 2 | 3 | 4 | 5 |
|---|---|---|---|---|---|
| **Confident** | ◯ | ◯ | ◯ | ◯ | ◯ |
| **Creative** | ◯ | ◯ | ◯ | ◯ | ◯ |
| **Confused** | ◯ | ◯ | ◯ | ◯ | ◯ |
| **Guided towards a good solution** | ◯ | ◯ | ◯ | ◯ | ◯ |
| **Productive** | ◯ | ◯ | ◯ | ◯ | ◯ |
| **Slowed down** | ◯ | ◯ | ◯ | ◯ | ◯ |

7. I found the tool... *

*Mark only one oval per row.*

| | 1 | 2 | 3 | 4 | 5 |
|---|---|---|---|---|---|
| **Easy-to-use** | ◯ | ◯ | ◯ | ◯ | ◯ |
| **Good fit for the purpose** | ◯ | ◯ | ◯ | ◯ | ◯ |
| **Intuitive** | ◯ | ◯ | ◯ | ◯ | ◯ |
| **Slow** | ◯ | ◯ | ◯ | ◯ | ◯ |
| **Visually appealing** | ◯ | ◯ | ◯ | ◯ | ◯ |

8. I found the recommendations.... *

*Mark only one oval per row.*

| | 1 | 2 | 3 | 4 | 5 |
|---|---|---|---|---|---|
| **Complete** | ◯ | ◯ | ◯ | ◯ | ◯ |
| **Confusing** | ◯ | ◯ | ◯ | ◯ | ◯ |
| **Correct** | ◯ | ◯ | ◯ | ◯ | ◯ |
| **Credible** | ◯ | ◯ | ◯ | ◯ | ◯ |
| **Inconsistent** | ◯ | ◯ | ◯ | ◯ | ◯ |
| **Intuitive** | ◯ | ◯ | ◯ | ◯ | ◯ |
| **Useful** | ◯ | ◯ | ◯ | ◯ | ◯ |

*Skip to question 12*

## Automatic suggestions

On a scale of 1 to 5, where 1 is the lowest value and 5 the highest value, please, respond to the following question.

9. During the experiment, I felt... *

*Mark only one oval per row.*

| | 1 | 2 | 3 | 4 | 5 |
|---|---|---|---|---|---|
| **Confident** | ◯ | ◯ | ◯ | ◯ | ◯ |
| **Creative** | ◯ | ◯ | ◯ | ◯ | ◯ |
| **Confused** | ◯ | ◯ | ◯ | ◯ | ◯ |
| **Guided towards a good solution** | ◯ | ◯ | ◯ | ◯ | ◯ |
| **Productive** | ◯ | ◯ | ◯ | ◯ | ◯ |
| **Slowed down** | ◯ | ◯ | ◯ | ◯ | ◯ |

10. I found the recommendations.... *

*Mark only one oval per row.*

| | 1 | 2 | 3 | 4 | 5 |
|---|---|---|---|---|---|
| **Complete** | ◯ | ◯ | ◯ | ◯ | ◯ |
| **Confusing** | ◯ | ◯ | ◯ | ◯ | ◯ |
| **Correct** | ◯ | ◯ | ◯ | ◯ | ◯ |
| **Credible** | ◯ | ◯ | ◯ | ◯ | ◯ |
| **Inconsistent** | ◯ | ◯ | ◯ | ◯ | ◯ |
| **Intuitive** | ◯ | ◯ | ◯ | ◯ | ◯ |
| **Stimulating (they gave me ideas I didn't have)** | ◯ | ◯ | ◯ | ◯ | ◯ |
| **Useful** | ◯ | ◯ | ◯ | ◯ | ◯ |
| **Well-timed (they appeared right when I expected them)** | ◯ | ◯ | ◯ | ◯ | ◯ |

11. I found the tool... *

*Mark only one oval per row.*

| | 1 | 2 | 3 | 4 | 5 |
|---|---|---|---|---|---|
| **Easy-to-use** | ⬭ | ⬭ | ⬭ | ⬭ | ⬭ |
| **Good fit for the purpose** | ⬭ | ⬭ | ⬭ | ⬭ | ⬭ |
| **Intuitive** | ⬭ | ⬭ | ⬭ | ⬭ | ⬭ |
| **Slow** | ⬭ | ⬭ | ⬭ | ⬭ | ⬭ |
| **Visually appealing** | ⬭ | ⬭ | ⬭ | ⬭ | ⬭ |

*Skip to question 12*

## General

12. Which features would you improve, and how?

_______________________________________________

_______________________________________________

_______________________________________________

_______________________________________________

_______________________________________________

13. What features did you miss?

_______________________________________________

14. Do you have any other remarks?

_______________________________________________
